# Supplementary material for: Anomalous Purcell decay of strongly driven inhomogeneous emitters coupled to a cavity
Source: arXiv:2309.16641 ancillary file (2024-03-07)
Supplement: Supplementary file 1 [file Anomalous_Purcell_decay_of_strongly_driven_inhomogeneous_emitters_coupled_to_a_cavity_SI.pdf]

**Supplementary Information for**  
**Anomalous Purcell decay of strongly driven inhomogeneous**  
**emitters coupled to a cavity**

Michael T. Solomon,<sup>†,‡,¶</sup> Martin Koppenhöfer,<sup>†</sup> Cheng Ji,<sup>†,‡</sup> Gregory D. Grant,<sup>†,‡</sup> Ignas  
Masiulionis,<sup>†,‡</sup> Sean E. Sullivan,<sup>‡,¶,#</sup> F. Joseph Heremans,<sup>‡,¶,†</sup> Supratik Guha,<sup>‡,†,¶</sup> David D.  
Awschalom,<sup>†,‡,¶,§</sup> Aashish A. Clerk,<sup>†,¶</sup> and Alan M. Dibos<sup>\*,||,⊥,¶</sup>

<sup>†</sup>*Pritzker School of Molecular Engineering, University of Chicago, Chicago, IL 60637*

<sup>‡</sup>*Materials Science Division, Argonne National Laboratory, Lemont, IL 60439*

<sup>¶</sup>*Center for Molecular Engineering, Argonne National Laboratory, Lemont, IL 60439*

<sup>§</sup>*Department of Physics, University of Chicago, Chicago, IL 60637, USA*

<sup>||</sup>*Nanoscience and Technology Division, Argonne National Laboratory, Lemont, IL 60439*

<sup>⊥</sup>*Center for Nanoscale Materials, Argonne National Laboratory, Lemont, IL 60439*

<sup>#</sup>*Current address: memQ Inc., Chicago, IL 60615*

E-mail: [adibos@anl.gov](mailto:adibos@anl.gov)

# 1 Additional experimental details

## 1.1 Inverse taper simulations

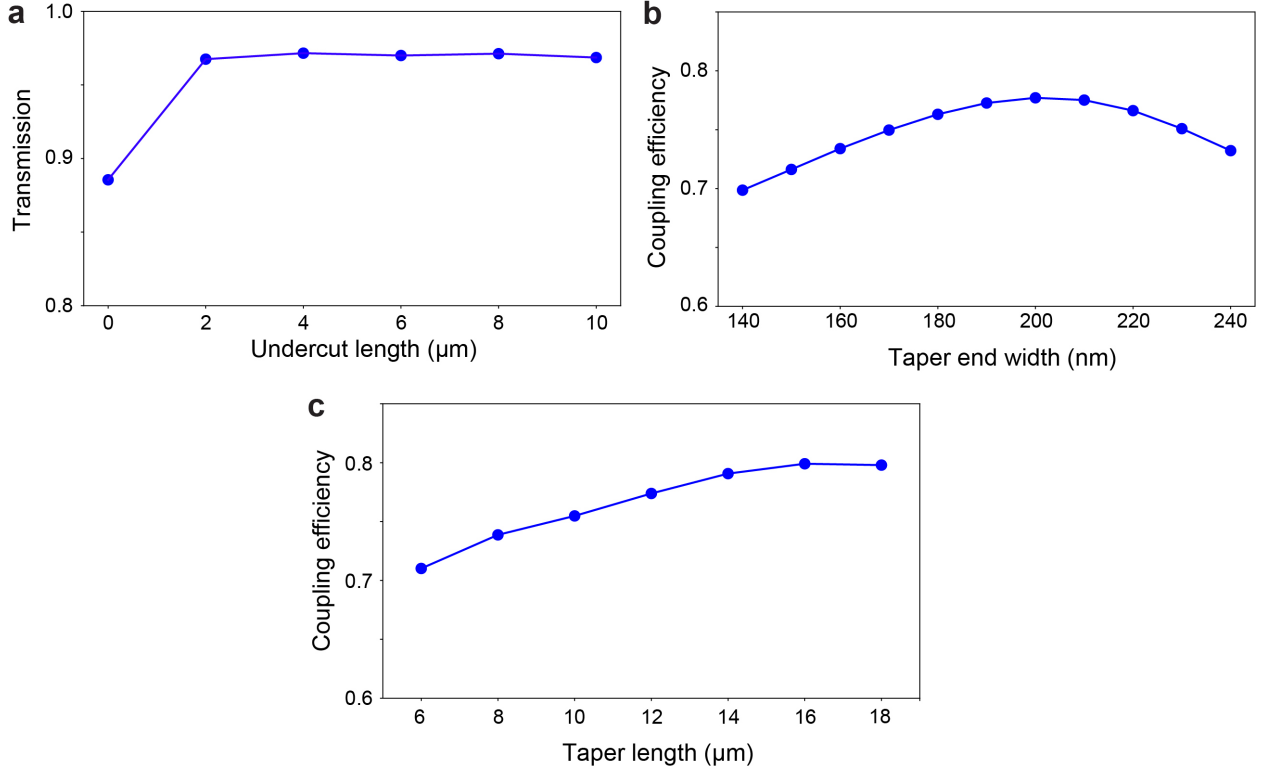

**Figure S1:** Inverse taper FDTD simulation results. (a) Guided mode transmission as light is routed in a Si waveguide from an undercut region to oxide region. (b) Fiber-to-waveguide coupling efficiency versus waveguide end facet width assuming a fixed taper length of 14  $\mu\text{m}$  and a fixed undercut of 4  $\mu\text{m}$ . (c) Fiber-to-waveguide coupling efficiency versus overall taper length width assuming a fixed endfacet width of 200 nm and a fixed undercut of 4  $\mu\text{m}$ .

In order to improve the lensed-fiber-to-waveguide coupling efficiency, we implemented a suspended inverse waveguide taper that protrudes off the edge of our sample. This approach is similar to the adiabatic inverse taper designs implemented previously for fully suspended 220 nm thick Si waveguides<sup>1</sup> and 250 nm thick Si waveguides.<sup>2</sup> For our simulations we ignored the presence of our  $\text{TiO}_2$  thin film, because it is only 30 nm thick and the refractive index is smaller than that of Si. In the simulations, we first assumed starting parameters similar to that in previous work: the end facet of the waveguide  $\sim 200 \text{ nm}^1$  and a taper length of  $\sim 14\mu\text{m}^2$  for mechanical stability of the tapered region. Then using 3D FDTD

(Lumerical), we investigated the minimum extent of the lateral undercut of the buried oxide layer that is needed to sufficiently guide light to the cavity. As shown in Figure S1a, as long as the initial undercut length is  $\geq 4\mu\text{m}$ , we don't lose much light as the mode transitions into the waveguide region in contact with the buried oxide layer. We then dithered around these values to further refine our end facet width (Fig. S1b) and taper length (Fig. S1c) for a fixed undercut length of  $4\mu\text{m}$ . To do so, we used a TE-polarized Gaussian source with a  $1.25\mu\text{m}$  waist radius placed  $14\mu\text{m}$  away from the end of the waveguide to mimic our commercial lensed fiber (OZ Optics) and simulated the transmitted power through a monitor along the waveguide  $4\mu\text{m}$  after the taper has reached a full width of  $650\text{ nm}$ . We can see that for a waveguide end facet width of  $\sim 200\text{ nm}$  and a taper length of  $14\mu\text{m}$  we have a maximum one-way coupling efficiency of  $\sim 80\%$  (Fig. S1b). Similarly, in Figure S1c, we can see that while an increased taper length has slightly higher coupling efficiency, for mechanical reasons we settle on the original taper length of  $14\mu\text{m}$ .

## 1.2 Nanofabrication process and cavity characterization

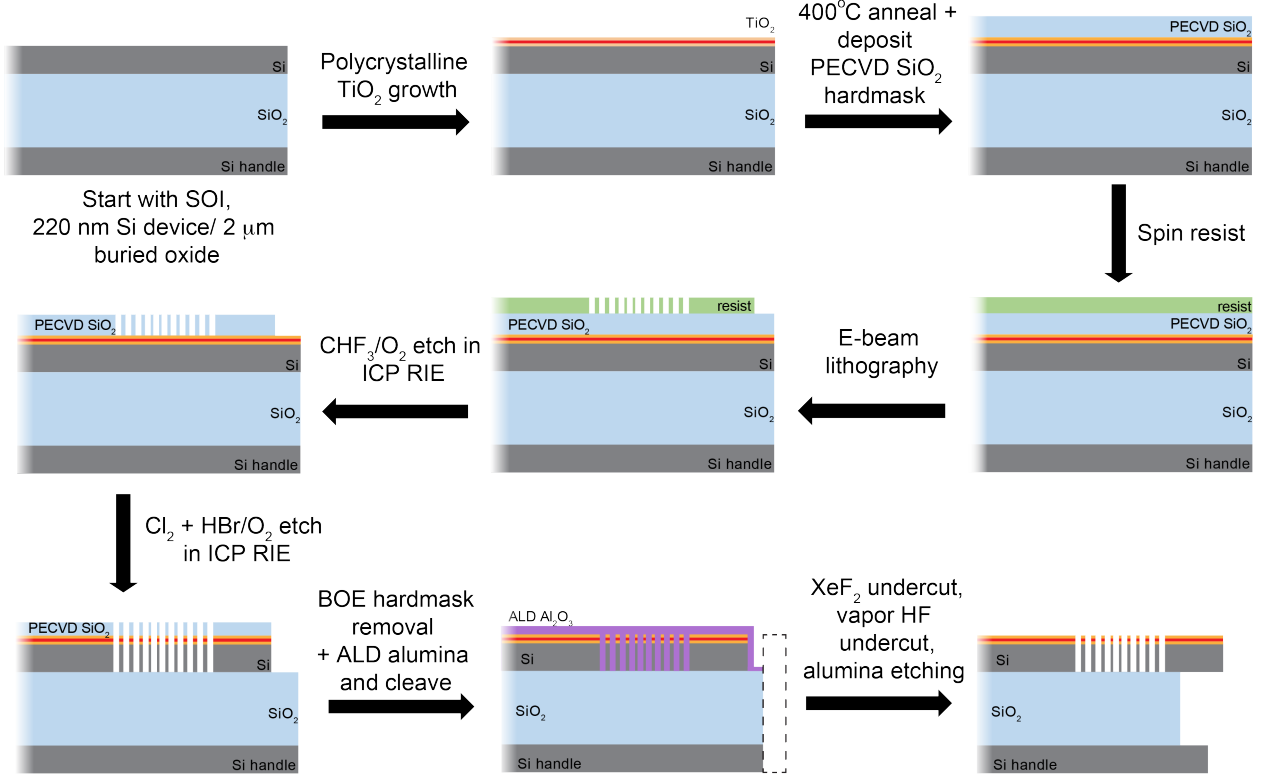

**Figure S2:** Full fabrication process flow for undercut waveguide devices.

The various fabrication steps to generate cavities and suspended inverse tapers are shown in Figure S2. All steps in the process flow are performed at the Center for Nanoscale Materials cleanroom at Argonne National Lab. Our  $\text{TiO}_2$  thin films are grown on silicon-on-insulator (SOI) substrates (Soitec) with a lightly boron-doped 220 nm thick Si device layer, 2  $\mu\text{m}$  buried oxide, and a more heavily boron-doped Si handle to reduce charging during subsequent fabrication steps. It is important to note that we deposit a device protection layer consisting of 200 cycles (20 nm) of thermal ALD alumina at a temperature of 175°C because polymeric resist layers do not provide sufficient protection, especially during the vapor HF step. We use this thickness and growth temperature of the alumina layer to mitigate pinholes that would allow the vapor etchants to attack the device layers during the undercut. Immediately after cleaving (Lattice Ax), we isotropically etch the Si handle layer

in a  $\text{XeF}_2$  vapor etch tool, which is what gives sample a scalloped edge (Fig. 2b-c in the main text). A long delay between the cleaving step and  $\text{XeF}_2$  etch process enables the formation of native oxide on the freshly cleaved Si surface, thereby slowing the otherwise deterministic etch rate of Si with  $\text{XeF}_2$ . After the Si handle undercut step, we then perform vapor HF etching (SPTS uEtch system) to undercut the buried thermal oxide layer. It is the order of these two vapor processes that gives the two-tiered undercut geometry shown in Figure S2a of the main text. We gently strip the alumina ALD layer using Aluminum etchant A (Transene) at 40°C. Finally, to mitigate any potential detrimental defects introduced by the various nanofabrication processes, we anneal the devices in pure  $\text{O}_2$  at 400°C using a rapid thermal annealing system (Annealsys). As discussed in Section 1.1, while our simulations suggest that longer tapers ( $> 14 \mu\text{m}$ ) have a slight improvement in the coupling efficiency, they also become much more fragile during the VHF undercut process because of strain in the suspended  $\text{SiO}_2$  and alumina layers after the Si handle undercut.

In order to compensate for run-to-run etch rate variations, our fabricated devices are designed to have a deliberate elliptical hole size parameter sweep, and so the cavity resonances on each chip range from 1510-1550 nm. Since we are coupling to the Er:rutile  $\text{TiO}_2$  transition at 1520.52 nm, the ideal device resonances are approximately 1530-1532 nm at room temperature to account for the 12 nm resonance blueshift when cooled to 3.5 K. We also know from experience that the cavity Q is limited by scattering loss from fabrication imperfections, so we can use the various visibility parameters in the reflection scan to estimate the waveguide-cavity coupling efficiency ( $\eta = 34\%$ ). Once we know the cavity resonance, we can detune the laser and measure the reflected laser power from the cavity. Comparing this value to the input power provides an estimate of the one-way fiber-to-waveguide coupling efficiency, this critical parameter doesn't affect later comparison with simulations, but it does determine output photon count rate and hence the experimental integration time needed for good enough signal-to-noise to enable lifetime fitting. We choose the highest laser power in our optical experiments ( $\phi = 1.1 \times 10^4$ ) to be below the threshold where the Si portion

of the cavity heats due to 2-photon absorption (and blueshifts the cavity resonance via gas desorption)<sup>3</sup> when CW laser excitation is incident at 3.5 K.

### 1.3 Cavity-coupled transient spectral hole burning measurements

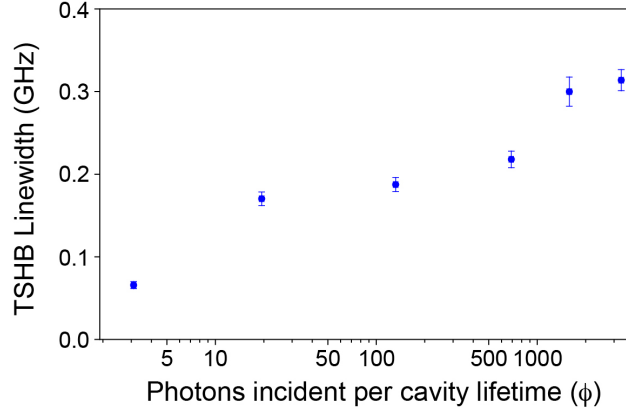

**Figure S3:** Cavity-coupled transient spectral hole burning (TSHB) measurements as a function of input photon flux at 3.5 K.

We use transient spectral hole burning (TSHB) measurements to get an upper bound on the homogeneous linewidth for the sub-ensemble of ions that couples to the optical cavity.<sup>4</sup> For this measurement we use a similar laser pumping and collection sequence (Fig. 2a of the main text) as for the optical lifetime measurements (Fig. 2c-d of the main text) to probe the emitter linewidths on the relevant pumping timescales. The primary differences for the TSHB measurements are: (1) we sweep the laser sideband frequency via a electro-optic phase modulator (as discussed in prior work<sup>3,5</sup>), and (2) we use a reduced number of experimental shots ( $N_{shots}=500$  per carrier-sideband detuning frequency), which results in a shorter overall integration time. We do this because our primary concern is the change in fluorescence intensity as a function of carrier-sideband detuning as opposed to acquiring sufficient signal-to-noise for accurate lifetime fitting, and this allows us to integrate quickly enough to avoid the longer timescale intensity fluctuations discussed in Section 1.5. Also, because we are probing the ions that are coupled to the cavity resonance, we adjust the collected intensity to account for the Lorentzian cavity lineshape ( $\kappa=2.94 \pm 0.05$  GHz). The

resultant plot (Fig. S3) shows that the TSHB linewidth (HWHM) versus incident flux seems to saturate near 300 MHz, though we have no intensity contrast at the highest pump fluxes used for the experiments in Figures 2c-d of the main text because we are saturating the ions regardless of cavity-sideband detuning. This is supported by the saturation of the integrated intensity presented in Figure 2e of the main text. We assume that at higher pump fluxes that we are likely still in this range, which is narrower than the cavity linewidth and so the ions coupled to the cavity are still in the ‘bad cavity limit’ even for the highest pump powers used in the experiment.

## 1.4 Bare waveguide ensemble lifetime

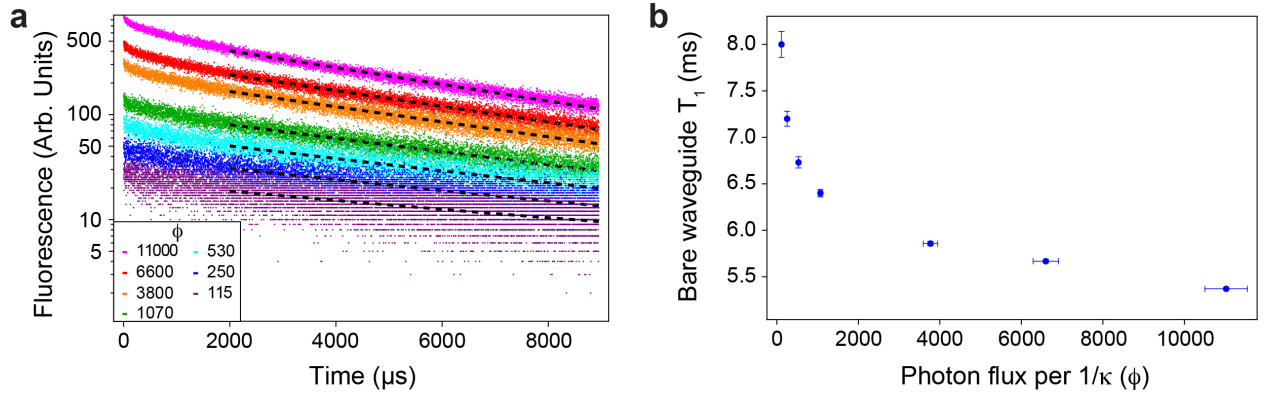

**Figure S4:** Optical lifetime ( $T_1$ ) estimates from Er ensembles coupled to bare waveguides. (a) A plot of the bare waveguide measured fluorescence decay curves for most of the incident fluxes shown in Figure 2d of the main text. The dashed black lines are single exponential fits. (b) The extracted single exponential optical lifetime ( $T_1$ ) values for the time traces in (a).

In order to determine a cavity-mediated decay rate enhancement, as shown in Figure 2d of the main text, we need to measure the decay rate ( $\Gamma_0 = 1/T_1$ ) of emitters in our devices without cavity-coupling. We use bare waveguides fabricated on the same chip as the nanocavities, that do not have etched holes but do have the same suspended inverse taper structures. Using the same pulse sequence depicted in Figure 2a of the main text with a resonant pump at  $\lambda = 1520.52$  nm (but with a longer collection time of 8.95 ms and  $N_{shots} = 10^5$  per incident flux), we obtain the fluorescence decay curves shown in Figure S4a. It is clear that

at higher incident powers the fluorescence has a slow exponential tail and a faster decaying component. This may be due to fabrication-induced recombination or other effects, but the origin isn't currently understood. Without knowing the origin of this effect, we don't know if these faster sub-ensembles will couple to the cavity mode. For simplicity, we extract a bare emitter lifetime using a single exponential fit to the slower exponential tail. The results of these single exponential fits are shown in Figure S4. We naively assume a single value of  $\Gamma_0 = 1/T_1$  in Figure 2d of the main text, using the exponential lifetime fit value of  $T_1 = 5.370 \pm 0.013$  ms extracted for the hardest optical drive at  $\phi \sim 11000$ . This value is in good agreement with  $T_1 = 5.25 \pm 0.03$  ms measured in previous work on Er implanted in rutile phase  $\text{TiO}_2$ .<sup>6</sup>

## 1.5 Integrated intensity measurements

Within our optical setup, we experience periodic intensity fluctuations on the timescale of 15-20 minutes. We suspect that the origin of these intensity fluctuations is because our fiber network is composed entirely of polarization maintaining (PM) fiber components with the exception of the lensed optical fiber which is machined from a conventional single mode fiber (OZ Optics). The polarization injected into the lensed fiber is rotated via a motorized fiber polarization controller (Phoenix Photonics) and set at the beginning of each experiment to match the TE-like polarization of our cavity devices at 3.5 K. During the measurements, likely due to fiber strain induced by thermal gradients within the cryostat when cold (we do not see these effects when warm), there is a modest modification of the polarization within the fiber affecting the injection power into the cavity. More significant is that as photons are routed back through the network for detection, the  $\sim 22$  dB polarization rejection ratio of our PM fiber circulator (Thorlabs) affects the intensity transmitted for detection. These effects are why we perform five full sweeps over the incident power for a given detuning ( $\Delta_c$ ) and then average the resultant lifetime histograms (bin-by-bin). We then fit these averaged histograms to extract the stretched exponential time constants (for the experimental curves

within Figures 2c-d of the main text) and integrated intensity (Fig. S5). Overall, the time constant fitting is robust to these fluctuations but the detected intensity is not. We are attempting to solve this problem moving forward with spliced PM lensed fibers.

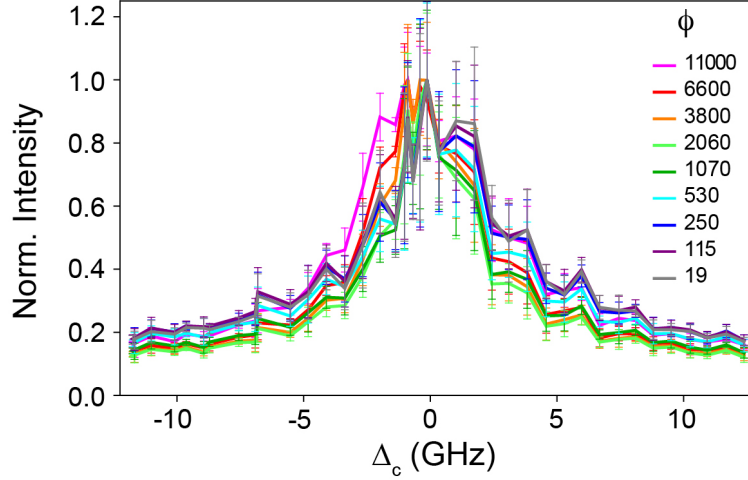

**Figure S5:** Normalized PLE intensity as a function of cavity detuning ( $\Delta_c$ ) for the various incident photon flux values (in units of photons per  $1/\kappa$ ). The error values for each data point come from the standard deviation in the integrated PLE intensity from the five measurements per detuning.

## 2 Additional simulation details

### 2.1 Integrated PLE from simulation values

To obtain a reference scale for the input flux  $\phi$  in our simulation, we consider the fluorescence of the spins for a resonant cavity,  $\Delta_c = 0$ . In the experiment, where the photon decay timescale  $1/\kappa$  is much shorter than the timescale on which the ions decay optically through the cavity, the fluorescence can be determined by integrating the number of photons impinging on the detector over the entire photon collection window. In our simulations, these two timescales are less clearly separated. Therefore, we consider a modified definition of the disorder-averaged fluorescence,

$$\overline{F_{\text{sub}}(t)} = \overline{F(t)} - \kappa_c |a(t_{\text{pulse}})|^2 e^{-\kappa(t-t_{\text{pulse}})}, \quad (1)$$

which subtracts the photons generated by the exponential decay of the initial state of the cavity field. An equivalent of the number of integrated counts (shown in Figure 2e of the main text) can now be obtained by integrating  $\overline{F_{\text{sub}}(t)}$  over the entire photon collection window,

$$\mathcal{F} = \int_{\text{collection window}} dt \overline{F_{\text{sub}}(t)} . \quad (2)$$

We fit  $\mathcal{F}$ , presented in Figure S6, to the PLE function given by Eq. (1) of the main text. For this fit function,  $\phi_0 = 1/p_2$  determines the critical photon flux at which saturation effects start to become relevant and serves as a reference scale that allows us to compare our experimental data set from Figure 2e of the main text with our numerical simulations.

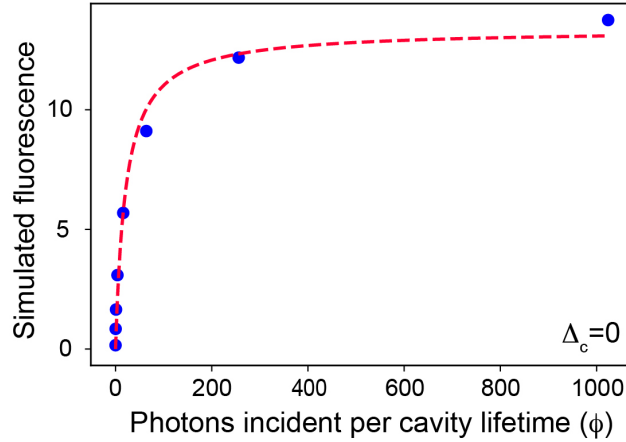

**Figure S6:** Simulated average PLE intensity a function of incident flux ( $\Delta_c=0$ ). Total fluorescence  $\mathcal{F}$  after subtracting the decay of the initial photon field, defined in Eq. (2), as a function of the input photon flux  $\phi$ . The dashed fit function represents the PLE function (Eq. (1) of the main text) and is used to determine the critical flux  $\phi_0$  where saturation effects start to become relevant.

## 2.2 Local decay model accounting for a modified cavity density of states

The effective model defined by Eqs. (16) to (18) of the main text assumes that the density of states of each auxiliary cavity is unchanged by the presence of the spins coupled to it. Given that CIT physics is able to renormalize the cavity density of states through the self-energy

term stemming from spins, cf. Eq. (9) of the main text, one may wonder if a more accurate description of the decay can be obtained if every spin locally decays with a decay rate that depends on the renormalized cavity density of states. This can be achieved by replacing the effective single-spin decay rate  $\gamma_{\text{eff},j}$  introduced in Eq. (13) of the main text by

$$\tilde{\gamma}_{\text{eff},j} = \gamma + \frac{\kappa g_j^2}{\left| i(\Delta_c - \delta_j) + \frac{\kappa}{2} - \sum_{k=1}^N \frac{g_j^2}{i(\delta_k - \delta_j) + \gamma/2} \right|^2} . \quad (3)$$

In this model, the relaxation of each spin is still local (i.e., non-collective), but the self-energy-term now introduces knowledge about the presence of all other spins (i.e., collective effects) into this local decay dynamics. We repeated the simulations performed for the local model defined in the main text with the modified dissipation rate (3) but found no significant deviations from the local model defined by Eq. (13) in the main text. Given the relatively small magnitude of the self-energy term compared to the bare cavity decay rate  $\kappa$ , such a result is to be expected.

### 2.3 Splitting of the peaks of the decay rate

As discussed in the main text, the ratio between the maximum decay rate at a given input flux  $\phi$  relative to the maximum decay rate at the lowest input flux is very different for the semiclassical and effective local models, and the semiclassical model matches well to the corresponding experimental data. In Figure S7, we show the dependence of the separation  $\Delta_+ - \Delta_-$  between the two peaks of the decay rate  $\Gamma$  as a function of  $\phi/\phi_0$ . We find that all three data sets agree in the regime  $\phi/\phi_0 \lesssim 1$ , where the range of detuning for which spins are highly depolarized to  $s_z^j \approx 0$  is much smaller than the finite extent  $\Delta_{\text{inh}}$  of the inhomogeneous frequency distribution. In the opposite regime  $\phi/\phi_0 \gg 1$ , the semiclassical and the effective local model deviate from the experimental measurements, likely because the ratio  $\Delta_{\text{inh}}/\kappa$  in the numerical simulations is much smaller than its corresponding value in the experiment.

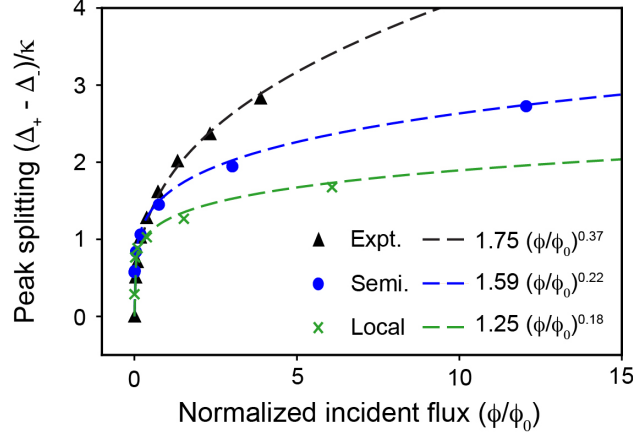

**Figure S7:** Separation of the two maxima ( $\Delta_{\pm}$ ) in the fluorescence decay rate  $\Gamma$  as a function of the photon flux ( $\phi$ ), normalized to the critical photon flux ( $\phi_0$ ) where saturation effects start to occur (see main text).

## References

- (1) Meenehan, S. M.; Cohen, J. D.; Gröblacher, S.; Hill, J. T.; Safavi-Naeini, A. H.; Aspelmeyer, M.; Painter, O. Silicon optomechanical crystal resonator at millikelvin temperatures. *Phys. Rev. A* **2014**, *90*, 011803.
- (2) Dibos, A. M.; Raha, M.; Phenicie, C. M.; Thompson, J. D. Atomic Source of Single Photons in the Telecom Band. *Physical Review Letters* **2018**, *120*, 243601–.
- (3) Dibos, A. M.; Solomon, M. T.; Sullivan, S. E.; Singh, M. K.; Sautter, K. E.; Horn, C. P.; Grant, G. D.; Lin, Y.; Wen, J.; Heremans, F. J.; Guha, S.; Awschalom, D. D. Purcell Enhancement of Erbium Ions in TiO<sub>2</sub> on Silicon Nanocavities. *Nano Letters* **2022**, *22*, 6530–6536.
- (4) Moerner, W. E., Ed. *Persistent Spectral Hole-Burning: Science and Applications*; Topics in Current Physics; Springer Berlin Heidelberg: Berlin, Heidelberg, 1988; Vol. 44; p 5.
- (5) Weiss, L.; Gritsch, A.; Merkel, B.; Reiserer, A. Erbium dopants in nanophotonic silicon waveguides. *Optica* **2021**, *8*, 40–41.
- (6) Phenicie, C. M.; Stevenson, P.; Welinski, S.; Rose, B. C.; Asfaw, A. T.; Cava, R. J.;

Lyon, S. A.; de Leon, N. P.; Thompson, J. D. Narrow Optical Line Widths in Erbium Implanted in TiO<sub>2</sub>. *Nano Letters* **2019**, *19*, 8928–8933.
